# Supplementary material for: Low-Energy On-Device Personalization for MCUs
Source: arXiv:2403.08040 source file (2024-10-01)
Supplement: Supplementary file 1 [file 8-Appendix.tex]

\newpage
\onecolumn
\begin{appendix}
\section{Appendix} % This will be labeled as 'Appendix A'
\label{sec:appendix}

\subsection{CloudML \& TinyML} % This will be labeled as 'Appendix A.1'
\label{sec:appendix1}

\begin{table}[h]
\centering
\footnotesize
\caption{Comparison of hardware devices}
\label{tab:Platform}
\begin{tabular}{@{}cccc@{}}
\toprule
Platform & Processor & Memory & Storage \\ 
\midrule
\begin{tabular}[c]{@{}c@{}} \textbf{Cloud-based}\\ NVIDIA \\ RTX 3090\end{tabular} & \begin{tabular}[c]{@{}c@{}}GPU \\ Nvidia Volta\end{tabular} & \begin{tabular}[c]{@{}c@{}}HBM \\ 24GB\end{tabular}  & \begin{tabular}[c]{@{}c@{}}SSD/Disk \\ TB$\sim$PB\end{tabular} \\
\midrule
\begin{tabular}[c]{@{}c@{}} \textbf{Mobile-based}\\ Smart Phone\end{tabular} & \begin{tabular}[c]{@{}c@{}}CPU \\ Mobile CPU\end{tabular}   & \begin{tabular}[c]{@{}c@{}}DRAM \\ 4GB\end{tabular}  & \begin{tabular}[c]{@{}c@{}}Flash \\ 64GB\end{tabular} \\
\midrule
\begin{tabular}[c]{@{}c@{}} \textbf{Mobile-based}\\ Raspberry Pi \\ 4 Model B\end{tabular} & \begin{tabular}[c]{@{}c@{}}CPU\\ Mobile CPU\end{tabular}    & \begin{tabular}[c]{@{}c@{}}DRAM\\ 4GB\end{tabular}   & \begin{tabular}[c]{@{}c@{}}SD Card \\ 4GB$\sim$128GB\end{tabular} \\
\midrule
\begin{tabular}[c]{@{}c@{}} \textbf{MCU-based}\\ STM32\\ L4R7ZI\end{tabular} & \begin{tabular}[c]{@{}c@{}}MCU \\ Arm Coretex-M4\end{tabular}       & \begin{tabular}[c]{@{}c@{}}SRAM\\ 640KB\end{tabular} & \begin{tabular}[c]{@{}c@{}}Flash\\ 2MB\end{tabular} \\
\midrule
\begin{tabular}[c]{@{}c@{}} \textbf{MCU-based}\\ STM32\\ H7A3ZI\end{tabular} & \begin{tabular}[c]{@{}c@{}}MCU \\ Arm Coretex-M7\end{tabular}    & \begin{tabular}[c]{@{}c@{}}SRAM\\ 1.18MB\end{tabular} & \begin{tabular}[c]{@{}c@{}}Flash\\ 2MB\end{tabular} \\
\bottomrule
\end{tabular}
\vskip -0.2in
\end{table}

\subsection{Initial Experiment: Personalization Performance of the Binary Supervised Model}
\label{sec:appendix2}
We conduct an initial experiment to verify the personalization performance of a binary supervised model. The initial experimental results show that the accuracy of the binary supervised model decreases on average from 66.59\% (on the target dataset) to 5.50\% (on the non-target datasets), which means it does not have a general feature extractor and the personalization performance is not ideal.

We employ supervised learning on the DeepFish \cite{saleh2020realistic} dataset to train a binary classification model (with/without fish) by ProxylessNAS. Subsequently, we employ pruning to compress the model, simulating its deployment on an MCU. The original classifier of this model is deleted, while the feature extractor is retained. We proceed to assess the model's accuracy across four distinct datasets using three different classifiers. 

Fig.~\ref{fig:app_initial_exp} shows the accuracy of the supervised model on the other datasets. The model exhibits an average accuracy of 66.59\% on its intended task, while it shows a decline in accuracy when presented with unseen data and new tasks. On the Pet, Bird, Plant, and Sea datasets, the average accuracy is reduced to 3.67\%, 0.85\%, 8.58\%, and 9.31\%. The results of the preliminary experiments indicate that supervised models are task-specific, and their feature extractors do not generalize well when dealing with unseen data and new tasks.

\begin{figure}[h]
% \vskip 0.2in
\begin{center}
\centerline{\includegraphics[width=0.4\textwidth]{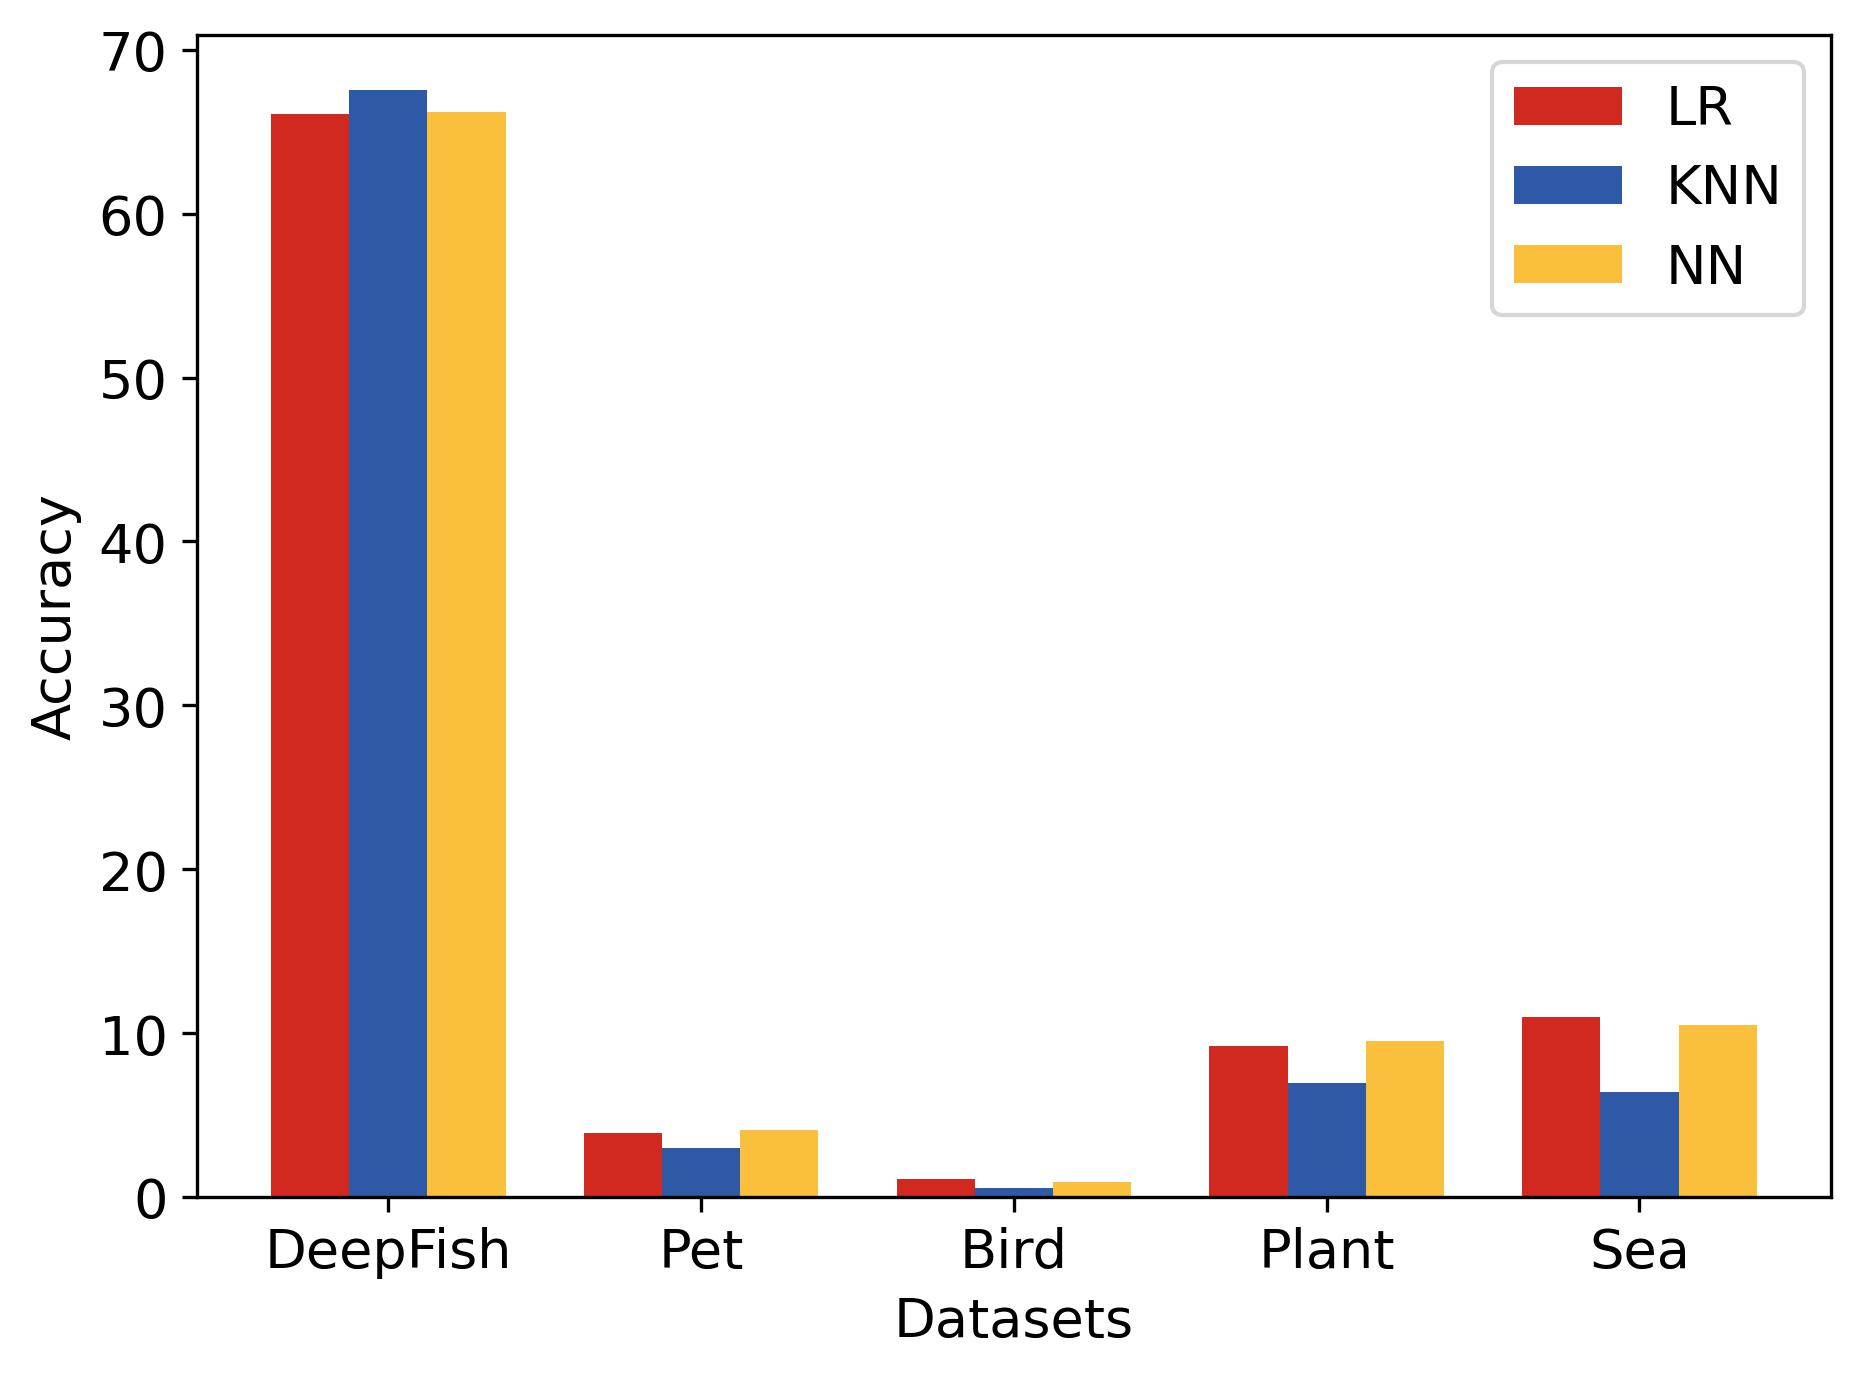}}
\caption{Accuracy of the supervised model on other datasets. }
\label{fig:app_initial_exp}
\end{center}
\vskip -0.2in
\end{figure}

\subsection{Personlization performance of the baseline and quantized PerEco}
\label{sec:appendix3}

% Please add the following required packages to your document preamble:
% \usepackage{multirow}
\begin{table*}[h]
\centering
\footnotesize
\caption{Personlization performance of the baseline and quantized PerEco}
\label{tab:app_exp3}
\begin{tabular}{|c|c|cccc|cccc|}
\hline
\multirow{2}{*}{\textbf{}} &
  \multirow{2}{*}{\textbf{Feature Extractor}} &
  \multicolumn{4}{c|}{\textbf{Dataset: Pet}} &
  \multicolumn{4}{c|}{\textbf{Dataset: Bird}} \\ \cline{3-10} 
 &
   &
  \multicolumn{1}{c|}{\textbf{LR}} &
  \multicolumn{1}{c|}{\textbf{KNN}} &
  \multicolumn{1}{c|}{\textbf{NN}} &
  \textbf{AVG} &
  \multicolumn{1}{c|}{\textbf{LR}} &
  \multicolumn{1}{c|}{\textbf{KNN}} &
  \multicolumn{1}{c|}{\textbf{NN}} &
  \textbf{AVG} \\ \hline
\multirow{4}{*}{BS} &

  Proxy\_0.3\_r224 &
  \multicolumn{1}{c|}{\begin{tabular}[c]{@{}c@{}}68.12±0.36 \end{tabular}} &
  \multicolumn{1}{c|}{\begin{tabular}[c]{@{}c@{}}61.69±0.69 \end{tabular}} &
  \multicolumn{1}{c|}{\begin{tabular}[c]{@{}c@{}}73.17±0.0.44 \end{tabular}} &
  \begin{tabular}[c]{@{}c@{}}67.66 \end{tabular} &
  \multicolumn{1}{c|}{\begin{tabular}[c]{@{}c@{}}39.91±0.41 \end{tabular}} &
  \multicolumn{1}{c|}{\begin{tabular}[c]{@{}c@{}}26.92±0.49 \end{tabular}} &
  \multicolumn{1}{c|}{\begin{tabular}[c]{@{}c@{}}43.85±0.36 \end{tabular}} &
  \begin{tabular}[c]{@{}c@{}}36.89 \end{tabular} \\ \cline{2-10} 

 &
  Proxy\_0.3\_r128 &
  \multicolumn{1}{c|}{\begin{tabular}[c]{@{}c@{}}47.56±1.10 \end{tabular}} &
  \multicolumn{1}{c|}{\begin{tabular}[c]{@{}c@{}}43.86±0.39 \end{tabular}} &
  \multicolumn{1}{c|}{\begin{tabular}[c]{@{}c@{}}55.30±0.71 \end{tabular}} &
  \begin{tabular}[c]{@{}c@{}}48.91\end{tabular} &
  \multicolumn{1}{c|}{\begin{tabular}[c]{@{}c@{}}23.12±0.98 \end{tabular}} &
  \multicolumn{1}{c|}{\begin{tabular}[c]{@{}c@{}}17.23±0.42 \end{tabular}} &
  \multicolumn{1}{c|}{\begin{tabular}[c]{@{}c@{}}27.83±0.97 \end{tabular}} &
  \begin{tabular}[c]{@{}c@{}}22.73 \end{tabular} \\ \cline{2-10} 
 &
  McuNet\_int3\_r224 &
  \multicolumn{1}{c|}{\begin{tabular}[c]{@{}c@{}}78.37±0.47 \end{tabular}} &
  \multicolumn{1}{c|}{\begin{tabular}[c]{@{}c@{}}75.34±1.21 \end{tabular}} &
  \multicolumn{1}{c|}{\begin{tabular}[c]{@{}c@{}}83.97±0.24 \end{tabular}} &
  \begin{tabular}[c]{@{}c@{}}79.23 \end{tabular} &
  \multicolumn{1}{c|}{\begin{tabular}[c]{@{}c@{}}45.84±0.63 \end{tabular}} &
  \multicolumn{1}{c|}{\begin{tabular}[c]{@{}c@{}}33.93±0.84 \end{tabular}} &
  \multicolumn{1}{c|}{\begin{tabular}[c]{@{}c@{}}52.44±0.77 \end{tabular}} &
  \begin{tabular}[c]{@{}c@{}}44.07 \end{tabular} \\ \cline{2-10} 

 &
  McuNet\_int3\_r128 &
  \multicolumn{1}{c|}{\begin{tabular}[c]{@{}c@{}}61.04±0.78 \end{tabular}} &
  \multicolumn{1}{c|}{\begin{tabular}[c]{@{}c@{}}62.57±0.55 \end{tabular}} &
  \multicolumn{1}{c|}{\begin{tabular}[c]{@{}c@{}}71.78±0.77 \end{tabular}} &
  \begin{tabular}[c]{@{}c@{}}65.13 \end{tabular} &
  \multicolumn{1}{c|}{\begin{tabular}[c]{@{}c@{}}30.17±0.55 \end{tabular}} &
  \multicolumn{1}{c|}{\begin{tabular}[c]{@{}c@{}}23.80±0.64 \end{tabular}} &
  \multicolumn{1}{c|}{\begin{tabular}[c]{@{}c@{}}36.93±0.59 \end{tabular}} &
  \begin{tabular}[c]{@{}c@{}}30.30 \end{tabular} \\ \hline
\multirow{4}{*}{PerEco} &
  Proxy\_0.3\_r224\_quant &
  \multicolumn{1}{c|}{\begin{tabular}[c]{@{}c@{}}84.85±0.23 \\ \textcolor{Green}{↑16.73}\end{tabular}} &
  \multicolumn{1}{c|}{\begin{tabular}[c]{@{}c@{}}80.17±0.18 \\ \textcolor{Green}{↑18.48}\end{tabular}} &
  \multicolumn{1}{c|}{\begin{tabular}[c]{@{}c@{}}83.51±0.28 \\ \textcolor{Green}{↑10.34}\end{tabular}} &
  \begin{tabular}[c]{@{}c@{}}82.84 \\ \textcolor{Green}{↑15.18}\end{tabular} &
  \multicolumn{1}{c|}{\begin{tabular}[c]{@{}c@{}}52.39±0.22 \\ \textcolor{Green}{↑12.48}\end{tabular}} &
  \multicolumn{1}{c|}{\begin{tabular}[c]{@{}c@{}}40.06±0.26 \\ \textcolor{Green}{↑13.14}\end{tabular}} &
  \multicolumn{1}{c|}{\begin{tabular}[c]{@{}c@{}}52.06±0.35 \\ \textcolor{Green}{↑8.21}\end{tabular}} &
  \begin{tabular}[c]{@{}c@{}}48.17\\ \textcolor{Green}{↑11.28}\end{tabular} \\ \cline{2-10} 
  
 &
  Proxy\_0.3\_r128\_quant &
  \multicolumn{1}{c|}{\begin{tabular}[c]{@{}c@{}}76.77±0.99 \\ \textcolor{Green}{↑29.21}\end{tabular}} &
  \multicolumn{1}{c|}{\begin{tabular}[c]{@{}c@{}}70.68±1.04 \\ \textcolor{Green}{↑26.82}\end{tabular}} &
  \multicolumn{1}{c|}{\begin{tabular}[c]{@{}c@{}}75.97±0.81 \\ \textcolor{Green}{↑20.67}\end{tabular}} &
  \begin{tabular}[c]{@{}c@{}}74.47 \\ \textcolor{Green}{↑25.56}\end{tabular} &
  \multicolumn{1}{c|}{\begin{tabular}[c]{@{}c@{}}38.83±0.42 \\ \textcolor{Green}{↑15.71}\end{tabular}} &
  \multicolumn{1}{c|}{\begin{tabular}[c]{@{}c@{}}29.28±0.57 \\ \textcolor{Green}{↑12.05}\end{tabular}} &
  \multicolumn{1}{c|}{\begin{tabular}[c]{@{}c@{}}40.37±0.71 \\ \textcolor{Green}{↑12.54}\end{tabular}} &
  \begin{tabular}[c]{@{}c@{}}36.16 \\  \textcolor{Green}{↑13.43}\end{tabular} \\ \cline{2-10} 
 &
  McuNet\_int3\_r224\_quant &
  \multicolumn{1}{c|}{\begin{tabular}[c]{@{}c@{}}87.20±0.29 \\ \textcolor{Green}{↑8.83}\end{tabular}} &
  \multicolumn{1}{c|}{\begin{tabular}[c]{@{}c@{}}85.40±0.23 \\ \textcolor{Green}{↑10.06}\end{tabular}} &
  \multicolumn{1}{c|}{\begin{tabular}[c]{@{}c@{}}89.41±0.42 \\ \textcolor{Green}{↑5.44}\end{tabular}} &
  \begin{tabular}[c]{@{}c@{}}87.34 \\  \textcolor{Green}{↑8.11}\end{tabular} &
  \multicolumn{1}{c|}{\begin{tabular}[c]{@{}c@{}}57.98±0.42 \\ \textcolor{Green}{↑12.14}\end{tabular}} &
  \multicolumn{1}{c|}{\begin{tabular}[c]{@{}c@{}}47.95±0.57 \\ \textcolor{Green}{↑14.02}\end{tabular}} &
  \multicolumn{1}{c|}{\begin{tabular}[c]{@{}c@{}}61.13±0.71 \\ \textcolor{Green}{↑8.69}\end{tabular}} &
  \begin{tabular}[c]{@{}c@{}}55.69\\ \textcolor{Green}{↑11.62}\end{tabular} \\ \cline{2-10} 

 &
  McuNet\_int3\_r128\_quant &
  \multicolumn{1}{c|}{\begin{tabular}[c]{@{}c@{}}78.35±0.29\\ \textcolor{Green}{↑17.31}\end{tabular}} &
  \multicolumn{1}{c|}{\begin{tabular}[c]{@{}c@{}}77.94±0.37\\ \textcolor{Green}{↑15.37}\end{tabular}} &
  \multicolumn{1}{c|}{\begin{tabular}[c]{@{}c@{}}83.13±0.10\\ \textcolor{Green}{↑11.35}\end{tabular}} &
  \begin{tabular}[c]{@{}c@{}}79.81\\ \textcolor{Green}{↑14.68}\end{tabular} &
  \multicolumn{1}{c|}{\begin{tabular}[c]{@{}c@{}}44.44±0.89 \\ \textcolor{Green}{↑14.278}\end{tabular}} &
  \multicolumn{1}{c|}{\begin{tabular}[c]{@{}c@{}}34.88±0.58\\ \textcolor{Green}{↑11.08}\end{tabular}} &
  \multicolumn{1}{c|}{\begin{tabular}[c]{@{}c@{}}49.81±0.57 \\ \textcolor{Green}{↑12.88}\end{tabular}} &
  \begin{tabular}[c]{@{}c@{}}43.04 \\ \textcolor{Green}{↑12.74}\end{tabular} \\ \hline
\multirow{2}{*}{\textbf{}} &
  \multirow{2}{*}{\textbf{Feature Extractor}} &
  \multicolumn{4}{c|}{\textbf{Dataset: Plant}} &
  \multicolumn{4}{c|}{\textbf{Dataset: Sea}} \\ \cline{3-10} 
 &
   &
  \multicolumn{1}{c|}{\textbf{LR}} &
  \multicolumn{1}{c|}{\textbf{KNN}} &
  \multicolumn{1}{c|}{\textbf{NN}} &
  \textbf{AVG} &
  \multicolumn{1}{c|}{\textbf{LR}} &
  \multicolumn{1}{c|}{\textbf{KNN}} &
  \multicolumn{1}{c|}{\textbf{NN}} &
  \textbf{AVG} \\ \hline
\multirow{4}{*}{BS} &
  Proxy\_0.3\_r224 &
  \multicolumn{1}{c|}{\begin{tabular}[c]{@{}c@{}}49.80±0.76\end{tabular}} &
  \multicolumn{1}{c|}{\begin{tabular}[c]{@{}c@{}}46.09±0.42\end{tabular}} &
  \multicolumn{1}{c|}{\begin{tabular}[c]{@{}c@{}}56.46±0.25\end{tabular}} &
  \begin{tabular}[c]{@{}c@{}}50.78\end{tabular} &
  \multicolumn{1}{c|}{\begin{tabular}[c]{@{}c@{}}62.17±0.90\end{tabular}} &
  \multicolumn{1}{c|}{\begin{tabular}[c]{@{}c@{}}57.45±0.72\end{tabular}} &
  \multicolumn{1}{c|}{\begin{tabular}[c]{@{}c@{}}68.15±0.56\end{tabular}} &
  \begin{tabular}[c]{@{}c@{}}62.59\end{tabular} \\ \cline{2-10}

 &
  Proxy\_0.3\_r128&
  \multicolumn{1}{c|}{\begin{tabular}[c]{@{}c@{}}42.05±0.62\end{tabular}} &
  \multicolumn{1}{c|}{\begin{tabular}[c]{@{}c@{}}41.85±0.34\end{tabular}} &
  \multicolumn{1}{c|}{\begin{tabular}[c]{@{}c@{}}51.70±0.31\end{tabular}} &
  \begin{tabular}[c]{@{}c@{}}45.20\end{tabular} &
  \multicolumn{1}{c|}{\begin{tabular}[c]{@{}c@{}}51.81±0.73\end{tabular}} &
  \multicolumn{1}{c|}{\begin{tabular}[c]{@{}c@{}}49.71±0.88\end{tabular}} &
  \multicolumn{1}{c|}{\begin{tabular}[c]{@{}c@{}}59.51±0.31\end{tabular}} &
  \begin{tabular}[c]{@{}c@{}}53.68\end{tabular} \\ \cline{2-10} 
 &
  McuNet\_int3\_r224 &
  \multicolumn{1}{c|}{\begin{tabular}[c]{@{}c@{}}53.01±1.36\end{tabular}} &
  \multicolumn{1}{c|}{\begin{tabular}[c]{@{}c@{}}48.49±1.49\end{tabular}} &
  \multicolumn{1}{c|}{\begin{tabular}[c]{@{}c@{}}61.39±1.35\end{tabular}} &
  \begin{tabular}[c]{@{}c@{}}54.30\end{tabular} &
  \multicolumn{1}{c|}{\begin{tabular}[c]{@{}c@{}}69.38±0.79\end{tabular}} &
  \multicolumn{1}{c|}{\begin{tabular}[c]{@{}c@{}}60.81±0.77\end{tabular}} &
  \multicolumn{1}{c|}{\begin{tabular}[c]{@{}c@{}}72.04±0.46\end{tabular}} &
  \begin{tabular}[c]{@{}c@{}}67.41\end{tabular} \\ \cline{2-10} 
 &
  McuNet\_int3\_r128 &
  \multicolumn{1}{c|}{\begin{tabular}[c]{@{}c@{}}47.64±0.83\end{tabular}} &
  \multicolumn{1}{c|}{\begin{tabular}[c]{@{}c@{}}42.87±1.62\end{tabular}} &
  \multicolumn{1}{c|}{\begin{tabular}[c]{@{}c@{}}54.88±0.86\end{tabular}} &
  \begin{tabular}[c]{@{}c@{}}48.46\end{tabular} &
  \multicolumn{1}{c|}{\begin{tabular}[c]{@{}c@{}}61.41±0.69\end{tabular}} &
  \multicolumn{1}{c|}{\begin{tabular}[c]{@{}c@{}}51.73±0.69\end{tabular}} &
  \multicolumn{1}{c|}{\begin{tabular}[c]{@{}c@{}}64.79±0.79\end{tabular}} &
  \begin{tabular}[c]{@{}c@{}}59.31\end{tabular} \\ \hline
\multirow{4}{*}{PerEco} &
  Proxy\_0.3\_r224\_quant &
  \multicolumn{1}{c|}{\begin{tabular}[c]{@{}c@{}}54.54±0.28\\ \textcolor{Green}{↑4.74}\end{tabular}} &
  \multicolumn{1}{c|}{\begin{tabular}[c]{@{}c@{}}48.46±0.52\\ \textcolor{Green}{↑2.37}\end{tabular}} &
  \multicolumn{1}{c|}{\begin{tabular}[c]{@{}c@{}}58.41±0.32\\ \textcolor{Green}{↑1.95}\end{tabular}} &
  \begin{tabular}[c]{@{}c@{}}53.80\\  \textcolor{Green}{↑3.02}\end{tabular} &
  \multicolumn{1}{c|}{\begin{tabular}[c]{@{}c@{}}72.70±0.76\\ \textcolor{Green}{↑10.53}\end{tabular}} &
  \multicolumn{1}{c|}{\begin{tabular}[c]{@{}c@{}}66.93±0.57\\ \textcolor{Green}{↑9.48}\end{tabular}} &
  \multicolumn{1}{c|}{\begin{tabular}[c]{@{}c@{}}73.48±0.48\\ \textcolor{Green}{↑5.33}\end{tabular}} &
  \begin{tabular}[c]{@{}c@{}}71.04\\  \textcolor{Green}{↑8.45}\end{tabular} \\ \cline{2-10} 
  
 &
  Proxy\_0.3\_r128\_quant &
  \multicolumn{1}{c|}{\begin{tabular}[c]{@{}c@{}}49.60±0.35\\ \textcolor{Green}{↑7.55}\end{tabular}} &
  \multicolumn{1}{c|}{\begin{tabular}[c]{@{}c@{}}43.83±0.40\\ \textcolor{Green}{↑1.98}\end{tabular}} &
  \multicolumn{1}{c|}{\begin{tabular}[c]{@{}c@{}}54.01±0.16\\ \textcolor{Green}{↑2.31}\end{tabular}} &
  \begin{tabular}[c]{@{}c@{}}49.15\\ \textcolor{Green}{↑3.95}\end{tabular} &
  \multicolumn{1}{c|}{\begin{tabular}[c]{@{}c@{}}67.68±0.53\\ \textcolor{Green}{↑15.87}\end{tabular}} &
  \multicolumn{1}{c|}{\begin{tabular}[c]{@{}c@{}}61.51±0.31\\ \textcolor{Green}{↑11.80}\end{tabular}} &
  \multicolumn{1}{c|}{\begin{tabular}[c]{@{}c@{}}68.88±0.44\\ \textcolor{Green}{↑9.37}\end{tabular}} &
  \begin{tabular}[c]{@{}c@{}}66.02\\ \textcolor{Green}{↑12.34}\end{tabular} \\ \cline{2-10} 
 &
  McuNet\_int3\_r224\_quant &
  \multicolumn{1}{c|}{\begin{tabular}[c]{@{}c@{}}57.97±0.23\\ \textcolor{Green}{↑4.96}\end{tabular}} &
  \multicolumn{1}{c|}{\begin{tabular}[c]{@{}c@{}}53.07±0.33\\ \textcolor{Green}{↑4.58}\end{tabular}} &
  \multicolumn{1}{c|}{\begin{tabular}[c]{@{}c@{}}64.82±0.43\\ \textcolor{Green}{↑3.43}\end{tabular}} &
  \begin{tabular}[c]{@{}c@{}}58.62\\ \textcolor{Green}{↑4.32}\end{tabular} &
  \multicolumn{1}{c|}{\begin{tabular}[c]{@{}c@{}}73.31±0.29\\ \textcolor{Green}{↑3.93}\end{tabular}} &
  \multicolumn{1}{c|}{\begin{tabular}[c]{@{}c@{}}70.76±0.71\\ \textcolor{Green}{↑9.95}\end{tabular}} &
  \multicolumn{1}{c|}{\begin{tabular}[c]{@{}c@{}}78.13±0.40\\ \textcolor{Green}{↑6.09}\end{tabular}} &
  \begin{tabular}[c]{@{}c@{}}74.07\\ \textcolor{Green}{↑6.66}\end{tabular} \\ \cline{2-10} 

 &
  McuNet\_int3\_r128\_quant &
  \multicolumn{1}{c|}{\begin{tabular}[c]{@{}c@{}}52.19±0.20\\ \textcolor{Green}{↑4.55}\end{tabular}} &
  \multicolumn{1}{c|}{\begin{tabular}[c]{@{}c@{}}47.38±0.95\\ \textcolor{Green}{↑4.51}\end{tabular}} &
  \multicolumn{1}{c|}{\begin{tabular}[c]{@{}c@{}}59.07±0.29\\ \textcolor{Green}{↑4.19}\end{tabular}} &
  \begin{tabular}[c]{@{}c@{}}52.88\\ \textcolor{Green}{↑4.42}\end{tabular} &
  \multicolumn{1}{c|}{\begin{tabular}[c]{@{}c@{}}70.62±0.33\\ \textcolor{Green}{↑9.21}\end{tabular}} &
  \multicolumn{1}{c|}{\begin{tabular}[c]{@{}c@{}}67.56±0.18\\ \textcolor{Green}{↑15.83}\end{tabular}} &
  \multicolumn{1}{c|}{\begin{tabular}[c]{@{}c@{}}74.25±0.47\\ \textcolor{Green}{↑9.46}\end{tabular}} &
  \begin{tabular}[c]{@{}c@{}}70.81\\ \textcolor{Green}{↑11.50}\end{tabular} \\ \hline
\end{tabular}
\\[2ex] 
 \textcolor{Green}{↑x} is the accuracy improvement of PerEco compared with the quantized baseline.
\end{table*}

\end{appendix}
